# Supplementary material for: Quantum fluctuations determine the spin-flop transition in hematite
Source: arXiv:2510.23412 source file (2025-10-27)
Supplement: Supplementary file 1 [file supplemental.pdf]

# Quantum fluctuations determine the spin-flop transition in hematite
# — Supplemental Material —


Tobias Dannegger,[1] Imre Hagymási,[2] Levente Rózsa,[2,3] and Ulrich Nowak[1]

[1]*Fachbereich Physik, Universität Konstanz, D-78457 Konstanz, Germany*
[2]*Department of Theoretical Solid State Physics, Institute for Solid State Physics and Optics, HUN-REN Wigner Research Centre for Physics, H-1121 Budapest, Hungary*
[3]*Department of Theoretical Physics, Institute of Physics, Budapest University of Technology and Economics, Műegyetem rkp. 3., H-1111 Budapest, Hungary*


## S1. SCALING PROCEDURES

As discussed in the main text, a rescaling of the classical parameters according to Eq. (2) leaves the spin-wave frequencies and the magnetic moment invariant. Since a quantum model differs in many aspects from a classical one, the way that the model parameters should be scaled for different quantum numbers is a matter of choice, and in the following we want to consider some alternative approaches.

Another common ansatz (cf., e.g., Ref. [1]) is to rescale spins with the corresponding spin length, $\boldsymbol{S} \rightarrow \boldsymbol{S}/\sqrt{S(S+1)}$, which means to scale the parameters as

$$\mathcal{J}^{\mathrm{q}}_{ij}(S) = \frac{\mathcal{J}^{\mathrm{c}}_{ij}}{S(S+1)},\ d^{\mathrm{q}}_2(S) = \frac{d^{\mathrm{c}}_2}{S(S+1)},\ d^{\mathrm{q}}_4(S) = \frac{d^{\mathrm{c}}_4}{[S(S+1)]^2}. \tag{S1}$$

This leaves the mean-field Néel temperature [2]

$$k_{\mathrm{B}}T_{\mathrm{N}} = \tfrac{1}{3}JS(S+1), \tag{S2}$$

with the Boltzmann constant $k_{\mathrm{B}}$ and the sum of the isotropic exchange constants $J$, invariant. This rescaling was used in Ref. [3] to study the deviations in the critical temperature from the mean-field critical temperature using a high-temperature expansion.

However, the critical temperature of three-dimensional magnets depends weakly on the anisotropy, which means that choosing a different rescaling for the anisotropy would not considerably modify the critical temperature. A different rescaling is also motivated by the fact that the on-site anisotropy becomes meaningless for $S = \frac{1}{2}$; for this reason, it was proposed in Ref. [4] to rescale the exchange terms by $S^2$ and the anisotropy by $S(S-\frac{1}{2})$. We also investigate the approach where we rescale the exchange interactions with $S(S+1)$ to retain the same critical temperature in mean-field theory, while keeping the scaling from Eq. (2) in the main text for the other parameters:

$$\mathcal{J}^{\mathrm{q}}_{ij}(S) = \frac{\mathcal{J}^{\mathrm{c}}_{ij}}{S(S+1)},\ d^{\mathrm{q}}_2(S) = \frac{d^{\mathrm{c}}_2}{S^2},\ d^{\mathrm{q}}_4(S) = \frac{d^{\mathrm{c}}_4}{S^4}. \tag{S3}$$

This approach is similar to Ref. [4] in the sense that the anisotropy coefficients are rescaled by a smaller factor than the exchange term.

## S2. QUANTUM HEISENBERG HAMILTONIAN

Replacing the $x$- and $y$-components of the spin operators in the quantum version of the spin Hamiltonian from Eq. (1) with the ladder operators $\hat{S}^{\pm}_i = \hat{S}^x_i \pm \mathrm{i}\hat{S}^y_i$ yields

$$\begin{aligned}\hat{\mathcal{H}} = -\tfrac{1}{2}\sum_{i\neq j}\Big[&(\tfrac{1}{4}J^{xx}_{ij} - \tfrac{\mathrm{i}}{4}J^{xy}_{ij} - \tfrac{\mathrm{i}}{4}J^{yx}_{ij} - \tfrac{1}{4}J^{yy}_{ij})\hat{S}^{+}_i\hat{S}^{+}_j \\ &+(\tfrac{1}{4}J^{xx}_{ij} + \tfrac{\mathrm{i}}{4}J^{xy}_{ij} - \tfrac{\mathrm{i}}{4}J^{yx}_{ij} + \tfrac{1}{4}J^{yy}_{ij})\hat{S}^{+}_i\hat{S}^{-}_j \\ &+(\tfrac{1}{4}J^{xx}_{ij} - \tfrac{\mathrm{i}}{4}J^{xy}_{ij} + \tfrac{\mathrm{i}}{4}J^{yx}_{ij} + \tfrac{1}{4}J^{yy}_{ij})\hat{S}^{-}_i\hat{S}^{+}_j \\ &+(\tfrac{1}{4}J^{xx}_{ij} + \tfrac{\mathrm{i}}{4}J^{xy}_{ij} + \tfrac{\mathrm{i}}{4}J^{yx}_{ij} - \tfrac{1}{4}J^{yy}_{ij})\hat{S}^{-}_i\hat{S}^{-}_j \\ &+(\tfrac{1}{2}J^{xz}_{ij} - \tfrac{\mathrm{i}}{2}J^{yz}_{ij})\hat{S}^{+}_i\hat{S}^{z}_j + (\tfrac{1}{2}J^{xz}_{ij} + \tfrac{\mathrm{i}}{2}J^{yz}_{ij})\hat{S}^{-}_i\hat{S}^{z}_j \\ &+(\tfrac{1}{2}J^{zx}_{ij} - \tfrac{\mathrm{i}}{2}J^{zy}_{ij})\hat{S}^{z}_i\hat{S}^{+}_j + (\tfrac{1}{2}J^{zx}_{ij} + \tfrac{\mathrm{i}}{2}J^{zy}_{ij})\hat{S}^{z}_i\hat{S}^{-}_j \\ &+(J^{zz}_{ij})\hat{S}^{z}_i\hat{S}^{z}_j\Big] \\ -\sum_i\Big[&d_2(\hat{S}^z_i)^2 + d_4(\hat{S}^z_i)^4 \\ &+\tfrac{1}{2}\mu(B^x - \mathrm{i}B^y)\hat{S}^{+}_i + \tfrac{1}{2}\mu(B^x + \mathrm{i}B^y)\hat{S}^{-}_i + \mu B^z\hat{S}^z_i\Big].\end{aligned} \tag{S4}$$

We represent this operator in the basis described in the main text to obtain the matrix form, which is a very sparse matrix, since the Hamiltonian is limited to two-spin interactions, making the use of matrix-free methods such as the Arnoldi algorithm very efficient.

## S3. MEAN-FIELD THEORY

Here, we discuss the two approaches to mean-field theory discussed in Fig. 4 of the main text. Following Ref. [5], we replace the quantum version of Eq. (1) by the mean-field Hamiltonian

$$\hat{\mathcal{H}}_{\mathrm{MF}} = \tfrac{1}{2}\sum_{i\neq j}\langle\hat{\boldsymbol{S}}^T_i\rangle\mathcal{J}_{ij}\langle\hat{\boldsymbol{S}}_j\rangle - \sum_i\big[d_2S^2_{i,z} + d_4S^4_{i,z} + \mu\boldsymbol{B}_{\mathrm{MF}}\cdot\boldsymbol{S}_i\big], \tag{S5}$$

with the mean field

$$\boldsymbol{B}_{\mathrm{MF}} = \frac{1}{\mu}\sum_j\mathcal{J}_{ij}\langle\hat{\boldsymbol{S}}_j\rangle + \boldsymbol{B}. \tag{S6}$$

Note that while this approach results in a single-site problem where the parameters $\langle\hat{\boldsymbol{S}}_i\rangle$ can be determined, the single-ion

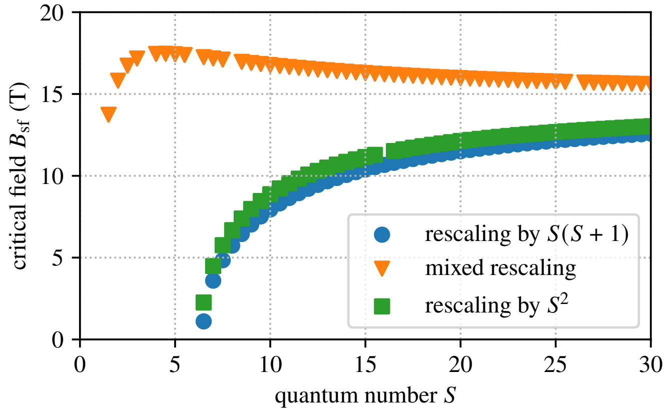


Figure S1. Mean-field calculated spin-flop field as a function of the quantum number for different scaling methods: blue circles: Eq. (S1); orange triangles: Eq. (S3); green squares: Eq. (2).

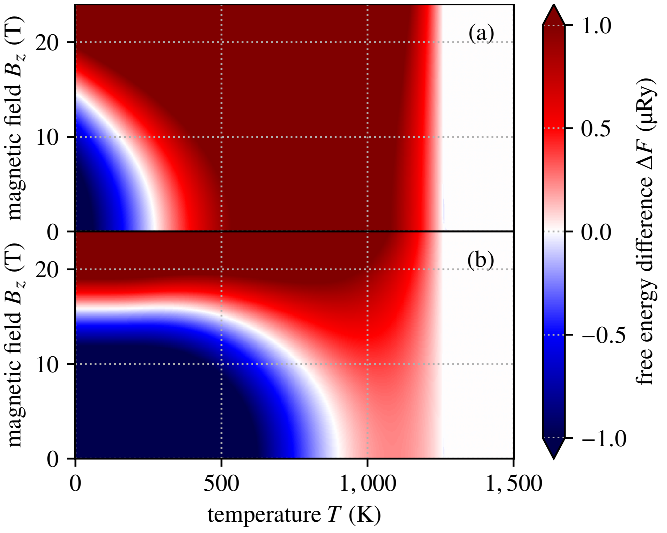


Figure S2. Calculated free-energy difference between the collinear antiferromagnetic and the flop phases, $F_{\mathrm{afm}} - F_{\mathrm{flop}}$, in the (a) classical and (b) quantum ($S = 2$) mean-field model with parameters scaled according to Eq. (S3).

anisotropy terms are not included in the mean field. This has important implications for the low-temperature behavior. In the antiferromagnetic state, the mean field is pointing along the $z$ direction, meaning that the spins being maximally polarized along the positive or negative $z$-axis are eigenstates of the Hamiltonian including the anisotropy terms, meaning that quantum fluctuations are absent in this state. However, in the weak ferromagnetic or spin-flop state the mean field has an in-plane component, and the mean-field term does not commute with the anisotropy terms. This means that the lowest-energy state will typically not be a maximally polarized spin eigenstate that would have a classical analogue, i.e., this approach takes on-site quantum fluctuations into account in the spin-flop phase.

In Fig. S1, we compare the behavior of the mean-field spin-flop transition as a function of the quantum number for different parameter scaling methods. We used the rescaling $\mu_{\mathrm{q}} = \mu_{\mathrm{cl}}/S$ in each approach to keep the atomic magnetic moment constant regardless of the spin quantum number; this appears to be the most consistent choice for ensuring a finite magnetic moment as $S \to \infty$ in the classical limit. For large quantum numbers $S$, the relative differences between all three scaling methods become arbitrarily small and approach the classical spin-flop field. For $S = \frac{1}{2}$, all three result in a spin-flop ground state, since the on-site anisotropy terms $d_2$ and $d_4$ stabilizing the antiferromagnetic state are not functional in this limit. In between, the critical field depends on the scaling method. When both the exchange and anisotropy parameters are scaled the same way [Eq. (2) or (S1)], we find a very similar behavior in both cases, with only slightly lower critical fields when the parameters are reduced more. With a mixed scaling according to Eq. (S3), we can keep the mean-field Néel temperature constant, while the critical spin-flop energy remains almost constant as well.

We use the latter scaling method to analyze the mean-field temperature dependence of the spin-flop field for $S = 2$. Figure S2 shows the difference in free energy between the antiferromagnetic phase (blue) and the spin-flop phase (red) for both the classical and the $S = 2$ quantum case. The free energy is calculated according to the procedure described in Ref. [5]. White color indicates a vanishing free-energy difference, which shows the boundary between the two phases at low temperature, and the paramagnetic phase at high temperature, where the expectation values $\langle \hat{S}_j \rangle$ are low. While the general shape of the phase boundary agrees very well with measurements in the quantum case and with atomistic spin dynamics simulations in the classical case, the actual values of the critical fields and temperatures are substantially different, with the exception of the classical spin-flop field at zero temperature, where the mean-field approximation becomes exact, and even an analytical solution can be derived.

Finally, we comment on the completely mean-field approach, where also the anisotropy terms in Eq. (S5) are incorporated in the mean field. In this case, the lowest-energy configuration will be a maximally polarized spin eigenstate at zero temperature in both the antiferromagnetic and the weak ferromagnetic phases, meaning that quantum fluctuations are completely absent. This results in a spin-flop field equal to its classical value for all quantum numbers $S$ when the rescaling in Eq. (2) is used. However, this does not lead to a qualitatively correct description at finite temperatures: the spin-flop field does not decrease linearly with the temperature in the classical case, and the Morin transition is usually absent. This implies that the fluctuations in the on-site anisotropy terms captured by Eq. (S5) are necessary for the qualitatively correct description of the temperature dependence mentioned above.

## S4. SPIN-WAVE THEORY

To derive the spin-wave approximation, we rewrite the anisotropy terms in the spin Hamiltonian in Eq. (S4) in tensorial

form as

$$\hat{\mathcal{H}} = -\tfrac{1}{2}\sum_{i,j}\hat{\boldsymbol{S}}_i^T\mathcal{J}_{ij}\hat{\boldsymbol{S}}_j - \sum_i \hat{\boldsymbol{S}}_i^T\mathcal{K}_i\hat{\boldsymbol{S}}_i - \sum_{i,\alpha,\beta,\gamma,\delta}\mathcal{K}_{i,4}^{\alpha\beta\gamma\delta}S_i^\alpha S_i^\beta S_i^\gamma S_i^\delta - \mu\sum_i \boldsymbol{B}^T\hat{\boldsymbol{S}}_i. \quad (S7)$$

First, we determine the classical ground state of the Hamiltonian by finding the unit vectors $\boldsymbol{S}_i^{(0)}$ satisfying

$$\boldsymbol{S}_i^{(0)} \times \frac{\partial\mathcal{H}}{\partial\boldsymbol{S}_i^{(0)}} = 0 \quad (S8)$$

at each lattice site, where $\mathcal{H}$ is the classical Hamiltonian (1). An approximate quantum ground state may be obtained by determining the low-energy excitations around this classical ground state within linear spin-wave theory. For this, we introduce a right-handed orthonormal basis $\{\boldsymbol{e}_{i,1}, \boldsymbol{e}_{i,2}, \boldsymbol{e}_{i,3} = \boldsymbol{S}_i^{(0)}\}$ at each lattice site, express the components of the spin operators in this basis, $\hat{S}_{i,\alpha} = \hat{\boldsymbol{S}}_i \cdot \boldsymbol{e}_{i,\alpha}$, and apply the linearized Holstein–Primakoff transformation [6],

$$\hat{S}_{i,1} = \sqrt{\tfrac{S}{2}}\big(\hat{a}_i + \hat{a}_i^\dagger\big),\ \hat{S}_{i,2} = -\mathrm{i}\sqrt{\tfrac{S}{2}}\big(\hat{a}_i - \hat{a}_i^\dagger\big),\ \hat{S}_{i,3} = S - \hat{a}_i^\dagger\hat{a}_i, \quad (S9)$$

where $S$ is the spin quantum number and $[\hat{a}_i, \hat{a}_j^\dagger] = \delta_{ij}$ are bosonic creation and annihilation operators. We define the rotation matrix $\boldsymbol{R}_i$ at site $i$ as $\boldsymbol{R}_i\tilde{\boldsymbol{S}}_i^{(0)} = \boldsymbol{S}_i^{(0)}$, where $\tilde{\boldsymbol{S}}_i^{(0)}$ points along the $z$-axis in the local coordinate system. We introduce the exchange tensor, single-site anisotropy tensor and magnetic field in the local coordinate system as

$$\tilde{\boldsymbol{B}}_i^T = \boldsymbol{B}_i^T\boldsymbol{R}_i,\ \tilde{\mathcal{J}}_{i,j} = \boldsymbol{R}_i^T\mathcal{J}_{i,j}\boldsymbol{R}_j,\ \tilde{\mathcal{K}}_i = \boldsymbol{R}_i^T\mathcal{K}_i\boldsymbol{R}_i,$$
$$\tilde{\mathcal{K}}_{i,4}^{\alpha\beta\gamma\delta} = \sum_{\alpha',\beta',\gamma',\delta'}\mathcal{K}_{i,4}^{\alpha'\beta'\gamma'\delta'}R_i^{\alpha'\alpha}R_i^{\beta'\beta}R_i^{\gamma'\gamma}R_i^{\delta'\delta}. \quad (S10)$$

The spin-wave Hamiltonian up to second-order terms in the creation and annihilation operators may be written as

$$\hat{\mathcal{H}} = E_0 + \hat{\mathcal{H}}_{\mathrm{SW}}, \quad (S11)$$

where

$$E_0 = -\tfrac{1}{2}\sum_{i,j}\tilde{\mathcal{J}}_{ij}^{zz}S(S+1) - \sum_i\tilde{\mathcal{K}}_i^{zz}S(S+1) - \sum_i\tilde{\mathcal{K}}_{i,4}^{zzzz}S^3(S+2) - \mu\sum_i\tilde{B}_i^z(S+\tfrac{1}{2}), \quad (S12)$$

and

$$\hat{\mathcal{H}}_{\mathrm{SW}} = \tfrac{1}{2}\sum_{i,j}\begin{bmatrix}\hat{a}_i^\dagger & \hat{a}_i\end{bmatrix}\begin{bmatrix}D_{0,i,j}+D_{\mathrm{nr},i,j} & D_{\mathrm{a},i,j}\\ D_{\mathrm{a},j,i}^* & D_{0,i,j}-D_{\mathrm{nr},i,j}\end{bmatrix}\begin{bmatrix}\hat{a}_j\\ \hat{a}_j^\dagger\end{bmatrix} \quad (S13)$$

is the harmonic spin-wave Hamiltonian containing the coefficients

$$D_{0,i,j} = -\frac{S}{2}\Big[\tilde{\mathcal{J}}_{ij}^{xx} + \tilde{\mathcal{J}}_{ij}^{yy} + \delta_{ij}2\Big(\tilde{\mathcal{K}}_i^{xx} + \tilde{\mathcal{K}}_i^{yy} + 6\tilde{\mathcal{K}}_{i,4}^{xxzz}S^2 + 6\tilde{\mathcal{K}}_{i,4}^{yyzz}S^2 - \sum_k\tilde{\mathcal{J}}_{ik}^{zz} - 2\tilde{\mathcal{K}}_i^{zz} - 4\tilde{\mathcal{K}}_{i,4}^{zzzz}S^2 - \mu\tilde{B}_i^z/S\Big)\Big], \quad (S14)$$

$$D_{\mathrm{nr},i,j} = -\frac{S}{2}\mathrm{i}\Big[\tilde{\mathcal{J}}_{ij}^{yx} - \tilde{\mathcal{J}}_{ij}^{xy} + \delta_{ij}2\Big(\tilde{\mathcal{K}}_i^{yx} - \tilde{\mathcal{K}}_i^{xy} + 6\tilde{\mathcal{K}}_{i,4}^{yxzz}S^2 - 6\tilde{\mathcal{K}}_{i,4}^{xyzz}S^2\Big)\Big], \quad (S15)$$

$$D_{\mathrm{a},i,j} = -\frac{S}{2}\Big[\tilde{\mathcal{J}}_{ij}^{xx} - \tilde{\mathcal{J}}_{ij}^{yy} + \mathrm{i}\Big(\tilde{\mathcal{J}}_{ij}^{yx} + \tilde{\mathcal{J}}_{ij}^{xy}\Big) + \delta_{ij}2\Big[\tilde{\mathcal{K}}_i^{xx} - \tilde{\mathcal{K}}_i^{yy} + 6\tilde{\mathcal{K}}_{i,4}^{xxzz}S^2 - 6\tilde{\mathcal{K}}_{i,4}^{yyzz}S^2 + \mathrm{i}\Big(\tilde{\mathcal{K}}_i^{yx} + \tilde{\mathcal{K}}_i^{xy} + 6\tilde{\mathcal{K}}_{i,4}^{yxzz}S^2 + 6\tilde{\mathcal{K}}_{i,4}^{xyzz}S^2\Big)\Big]\Big]. \quad (S16)$$

The energy in the uncorrelated state, defined as the vacuum of the bosonic operators $a_i|0\rangle = 0\ \forall i$, is

$$\langle 0|\hat{\mathcal{H}}|0\rangle = E_0 + \tfrac{1}{2}\,\mathrm{tr}(\boldsymbol{D}_0 - \boldsymbol{D}_{\mathrm{nr}}). \quad (S17)$$

Note that $\mathrm{tr}\,\boldsymbol{D}_{\mathrm{nr}} = 0$ since the nonreciprocal part of the matrix is antisymmetric. This coincides with the ground-state energy of the mean-field Hamiltonian (S5) in the collinear antiferromagnetic state. However, it differs from the mean-field energy in the weak ferromagnetic phase due to the non-commuting nature of the different terms in the Hamiltonian mentioned above.

A better approximation for the ground-state energy may be obtained in spin-wave theory from solving the equations of motion,

$$\partial_t\begin{bmatrix}\hat{a}_i\\ \hat{a}_i^\dagger\end{bmatrix} = -\frac{\mathrm{i}}{\hbar}\sum_j\sigma^z\begin{bmatrix}D_{0,i,j}+D_{\mathrm{nr},i,j} & D_{\mathrm{a},i,j}\\ D_{\mathrm{a},j,i}^* & D_{0,i,j}-D_{\mathrm{nr},i,j}\end{bmatrix}\begin{bmatrix}\hat{a}_j\\ \hat{a}_j^\dagger\end{bmatrix}, \quad (S18)$$

where $\sigma^z = \mathrm{diag}\,(1,-1)$ is a Pauli matrix. This can be diagonalized via the Bogoliubov transformation,

$$\begin{bmatrix}\hat{\alpha}_q\\ \hat{\alpha}_q^\dagger\end{bmatrix} = \sum_j\begin{bmatrix}V_{qj} & W_{qj}\\ W_{qj}^* & V_{qj}^*\end{bmatrix}\begin{bmatrix}\hat{a}_j\\ \hat{a}_j^\dagger\end{bmatrix}, \quad (S19)$$

resulting in $\mathrm{i}\partial_t\hat{\alpha}_q = \omega_q\hat{\alpha}_q$. Substituting the Bogoliubov transformation back into the Hamiltonian leads to

$$\hat{\mathcal{H}} = E_0 + \tfrac{1}{2}\sum_q\hbar\omega_q\big(\hat{\alpha}_q^\dagger\hat{\alpha}_q + \hat{\alpha}_q\hat{\alpha}_q^\dagger\big). \quad (S20)$$

The vacuum of the transformed operators, $\hat{\alpha}_q|0'\rangle = 0\ \forall k$, is an eigenvector of the Hamiltonian, and it has the energy

$$\langle 0'|\hat{\mathcal{H}}|0'\rangle = E_0 + \tfrac{1}{2}\,\mathrm{tr}\,\hbar\boldsymbol{\omega}, \quad (S21)$$

which is lower by $\frac{1}{2}\big[\mathrm{tr}(\hbar\boldsymbol{\omega}) - \mathrm{tr}(\boldsymbol{D}_0 - \boldsymbol{D}_{\mathrm{nr}})\big]$ than the uncorrelated energy calculated above. However, as shown in Fig. 4 of the main text, even the zero-point fluctuations are insufficient for a quantitatively correct description of the spin-flop field for $S = 2$ or $S = \frac{5}{2}$.

[1] L. Engelhardt, M. Luban, and C. Schröder, Finite quantum Heisenberg spin models and their approach to the classical limit, Phys. Rev. B **74**, 054413 (2006).
[2] C. Kittel, *Introduction to solid state physics*, 8th ed. (John Wiley & Sons, Hoboken, 2004).
[3] J. Oitmaa and W. Zheng, Curie and Néel temperatures of quantum magnets, J. Phys. Condens. Matter **16**, 8653 (2004).
[4] W. Yung-Li and H. B. Callen, Spin waves in the spin-flop phase of an antiferromagnet, and metastability of the spin-flop transition, J. Phys. Chem. Solids **25**, 1459 (1964).
[5] T. Dannegger, A. Deák, L. Rózsa, E. Galindez-Ruales, S. Das, E. Baek, M. Kläui, L. Szunyogh, and U. Nowak, Magnetic properties of hematite revealed by an *ab initio* parameterized spin model, Phys. Rev. B **107**, 184426 (2023).
[6] T. Holstein and H. Primakoff, Field dependence of the intrinsic domain magnetization of a ferromagnet, Phys. Rev. **58**, 1098 (1940).
